# Supplementary material for: Optical properties of superconducting pressurized LaH$_{10}$
Source: arXiv:2007.06640 source file (2020-07-13)
Supplement: Supplementary file 1 [file Supplementary_information_to_Optical_properties_of_superconducting.._Elatresh_et_al.pdf]

# Supporting Information Appendix
# For
# Optical properties of superconducting pressurized $LaH_{10}$

**S. F. Elatresh, T. Timusk, and E. J. Nicol**

## SI Text:

Table S1 presents the full structural optimization symmetry information for the LaH10-Fm3m phase at 210 GPa. Also, we calculated X-ray diffraction spectra (for wavelength 1.218 Å) for this structure at the same pressure (Fig. S1).

We enlarged the calculated density of states (DOS) for LaH10-Fm3m phase at 210 GPa near the Fermi level (Fig. S2). In addition, we calculated partial density of states for this structure at the same pressure (Fig. S3).

For useful comparison, we calculated the phonon density of states in unit of meV (Fig. S4).

We highlighted some of the important distances and showed their position in Fig. S5. To confirm that we did not miss anything, we performed atom to atom distances analysis. The La-La, H-H, and La-H distances are shown in Fig. S6,7,and 8, respectively.

**Table S1.** Lattice parameters and atomic positions for $LaH_{10}$ (Fm-3m) at 210 GPa.

| Compound | Pressure (GPa) | Space group | Lattice parameters, Å, degree | Atomic positions |
|---|---|---|---|---|
| $LaH_{10}$ | 210 | *Fm*-3*m* | $a=b=c=4.9296$<br>$\alpha = \beta = \gamma = 90°$ | *La 0.500 0.500 0.500*<br>*H 0.250 0.250 0.250*<br>*H 0.750 0.750 0.750*<br>*H 0.120 0.120 0.120*<br>*H 0.879 0.879 0.879*<br>*H 0.638 0.120 0.120*<br>*H 0.361 0.879 0.879*<br>*H 0.120 0.638 0.120*<br>*H 0.879 0.361 0.879*<br>*H 0.120 0.120 0.638*<br>*H 0.879 0.879 0.361* |

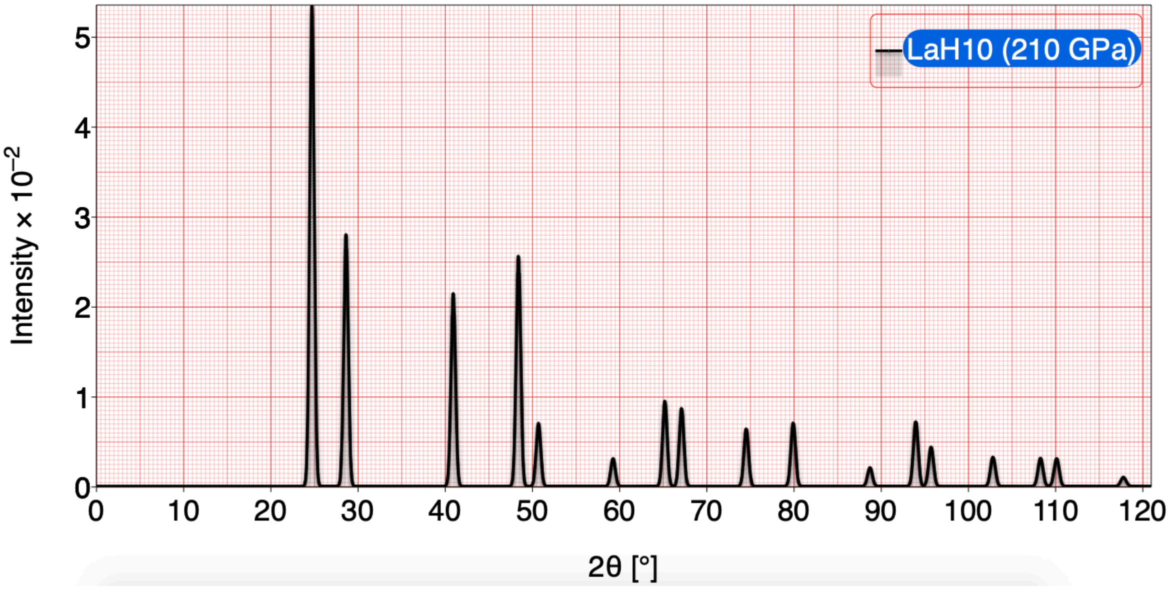


**Fig. S1:** Calculated X-ray diffraction spectra (for wavelength 1.218 Å) for $LaH_{10}$ (Fm-3m) at 210 GPa

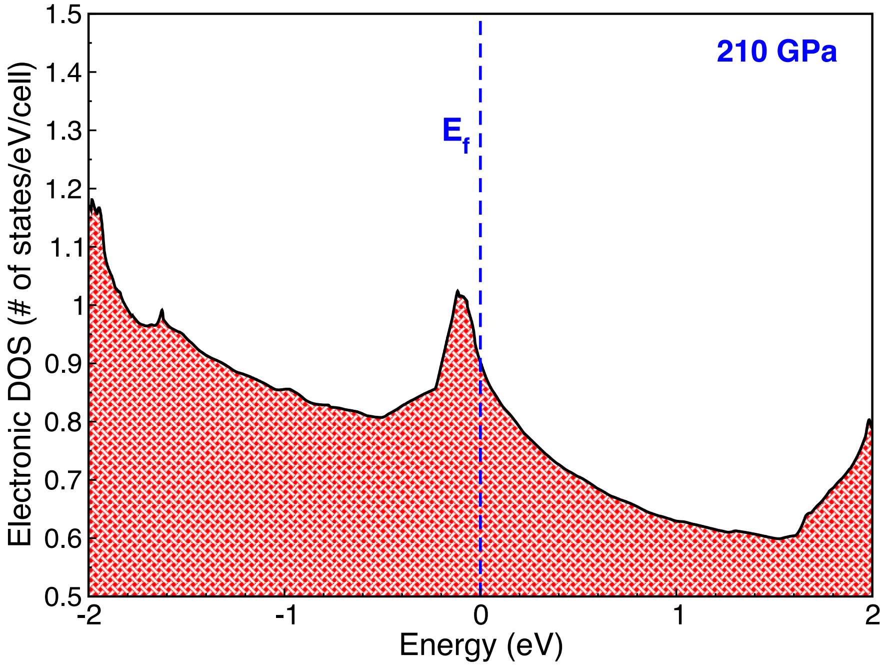


**Fig. S2:** Electronic density of states for $LaH_{10}$ (Fm-3m) at 210 GPa.

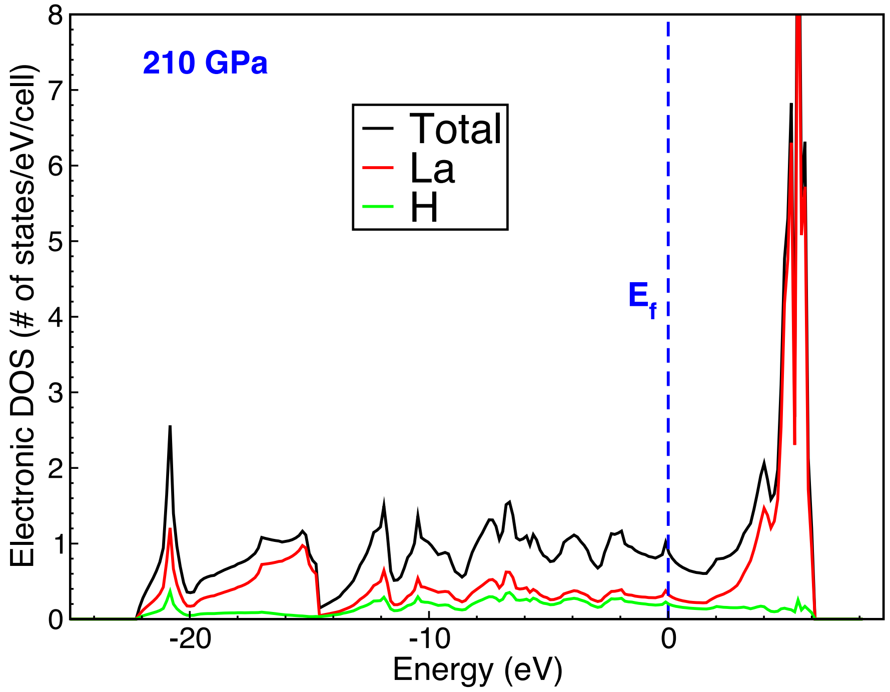


**Fig. S3**: Partial electronic density of states for $LaH_{10}$ (Fm-3m) at 210 GPa.

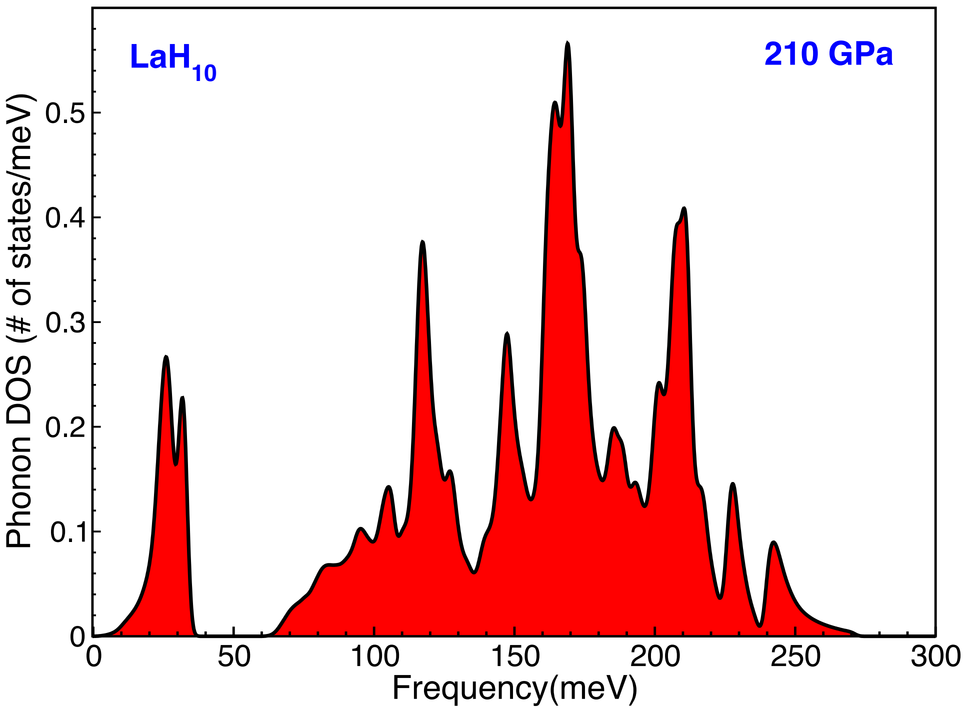


**Fig. S4:** Harmonic phonon density of states for $LaH_{10}$ (Fm-3m) at 210 GPa.

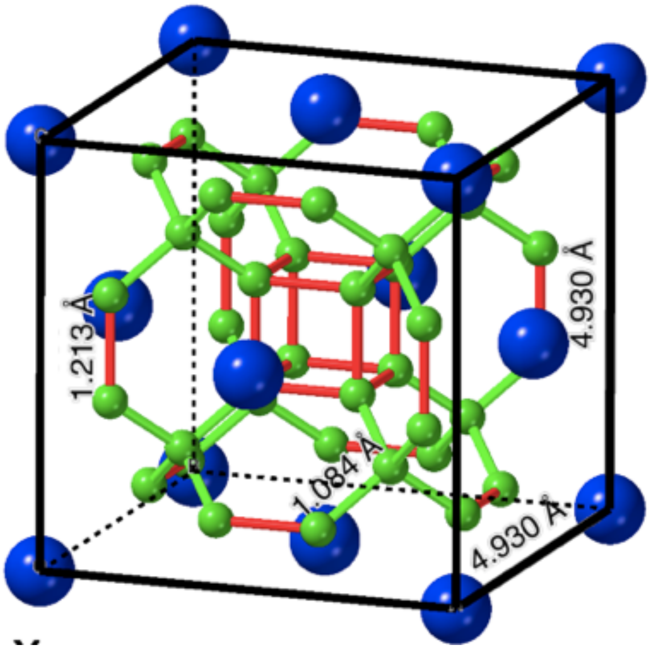


**Fig. S5:** Crystal structure for $LaH_{10}$ (Fm-3m) at 210 GPa.

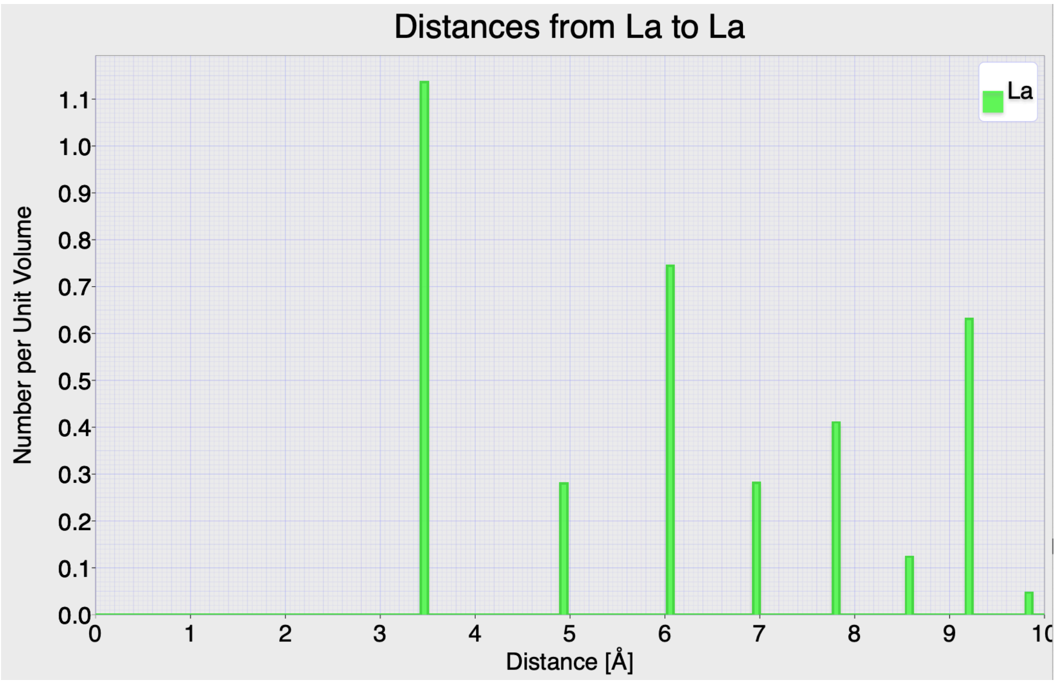


Fig. S6: Histograms of the distance of La to La for $LaH_{10}$ (Fm-3m) at 210 GPa.

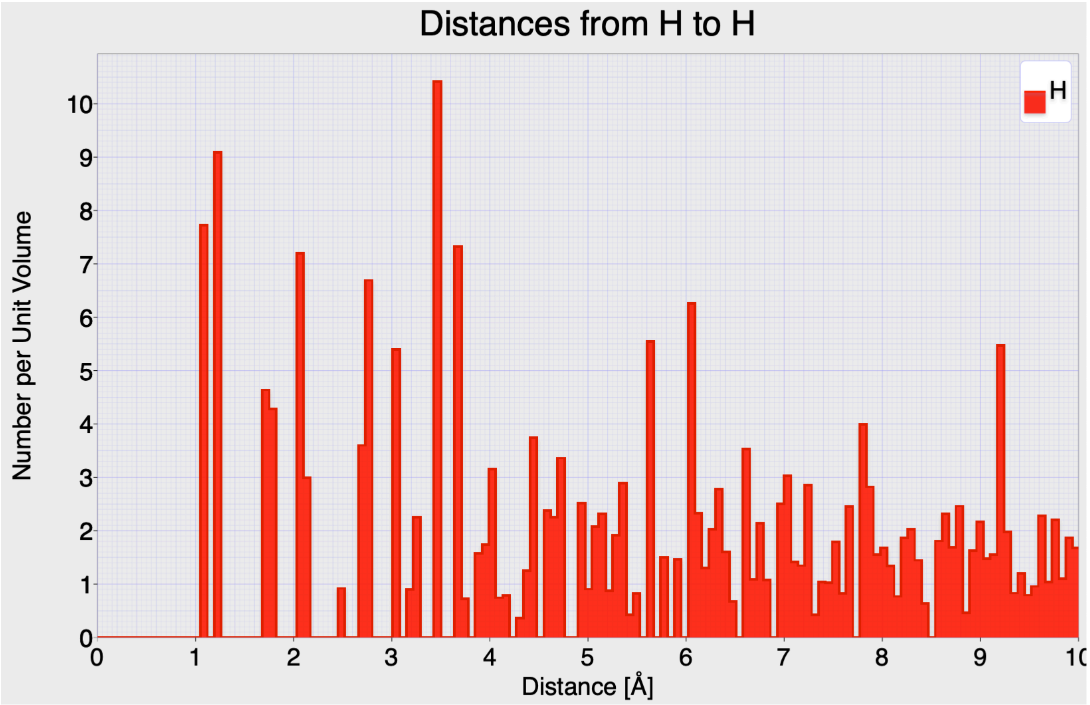


**Fig. S7:** Histograms of the distance of H to H for $LaH_{10}$ (Fm-3m) at 210 GPa.

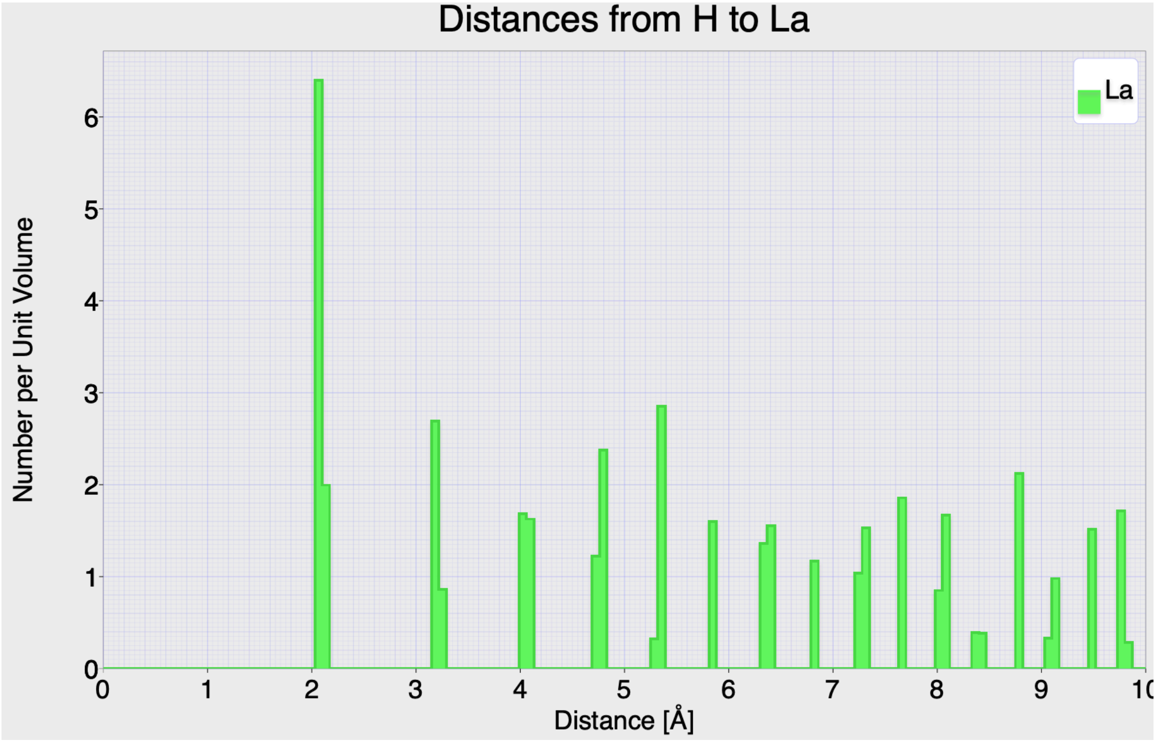


Fig. S8: Histograms of the distance of H to La for $LaH_{10}$ (Fm-3m) at 210 GPa.
